# Supplementary material for: Atlantis: Enabling Underwater Depth Estimation with Stable Diffusion
Source: arXiv:2312.12471 source file (2023-12-19)
Supplement: Supplementary file 1 [file X_suppl.tex]

\clearpage
\setcounter{page}{1}

\maketitlesupplementary

\setcounter{section}{0}
\setcounter{table}{0}
\setcounter{figure}{0}

In this supplementary material, we first provide quantitative results of another two depth models trained on our dataset, compared with their terrestrial pretrained counterparts. We also make comparisons with previous synthetic underwater depth dataset \cite{depth_uwgan} on training depth model. Then, we showcase examples of underwater images generated by our method alongside their corresponding terrestrial depth maps. Finally, we provide more visual results on unseen real underwater scenes from UIEB \cite{uieb2019li} and SQUID \cite{squid2020berman} datasets, as well as more underwater image enhancement results using Sea-thru algorithm \cite{seathur2019akkaynak}.

\section{More Quantitative Results}
In this section, we extend our analysis beyond iDisc \cite{idisc2023piccinelli} and NeWCRFs \cite{newcrfs2022yuan} from the main paper by training two additional methods, IEBins \cite{iebins} and VA-DepthNet \cite{vadepthnet}, on our dataset, Atlantis. Their performance is compared with their respective pretrained versions on terrestrial datasets. Quantitative evaluations on the Sea-thru \cite{seathur2019akkaynak} and SQUID \cite{squid2020berman} datasets are detailed in Tables \ref{tab:seathru} and \ref{tab:squid}. The results show that similar to iDisc and NeWCRFs, the pretrained versions of IEBins and VA-DepthNet struggle with real underwater datasets. However, significant improvements are observed when these models are trained on Atlantis. This enhancement in performance on unseen real underwater scenes further confirms the effectiveness of our dataset in training  state-of-the-art terrestrial depth models for underwater depth estimation, effectively narrowing the domain gap. Atlantis, with its realistic underwater imagery, accurate depth, vast diversity and theoretically unlimited scale of generation, offers a promising solution to the data scarcity challenge in underwater depth estimation.

\section{Comparisons with Depth Model Trained on GAN-based Dataset}
In this section, we compare the performance of depth models trained on our Atlantis dataset with that trained on GAN-based dataset \cite{depth_uwgan, uwcnn, uwgan2019wang}. We selected VA-DepthNet \cite{vadepthnet} for this comparative analysis. Due to the unavailability of the specific dataset proposed in \cite{depth_uwgan}, we utilized the dataset synthesized in the same pipeline in \cite{uwcnn}. This dataset comprises 14,490 images, generated from 10 water types based on NYU Depthv2 depth data. We train VA-DepthNet \cite{vadepthnet} following its default setting on NYU-Depthv2 dataset for 20 epochs. The quantitative results are listed in Table \ref{tab:gan}. We can find that the model trained on Atlantis consistently outperforms that trained on the GAN-based dataset across most metrics, particularly when evaluated on the SQUID dataset \cite{squid2020berman}. This suggests that while GAN-based dataset can partially reduce the domain gap by simulating underwater color casts, it falls short in capturing the full complexity of underwater scenes. In contrast, Atlantis excels in generating diverse and vivid underwater scenes with a variety of color casts, turbidity levels, and textures. This diversity enables depth models to generalize more effectively to unseen underwater environments, highlighting the superiority of Atlantis in underwater depth estimation.

\section{More Samples in Atlantis}
Here, we present additional examples from our underwater depth dataset, Atlantis, along with the depth maps used for image generation in Figure \ref{fig:sample}. These samples highlight the effectiveness of our dataset in maintaining the structure of the original depth maps while introducing a diverse range of underwater textures, lighting conditions, and color casts in the generated images. The realistic and varied underwater scenes, coupled with corresponding accurate depth maps, are instrumental in training state-of-the-art depth estimation models specifically for underwater applications and improve their performance on unseen real underwater images. In the future, we may further improve the quality of our dataset by involving more and diverse underwater scenes for ControlNet pretraining, bridging the gap between relative and absolute depth, and expanding the number of training samples available.

\begin{table*}[!t]\footnotesize
	\caption{Quantitative comparisons on real underwater images from D3 and D5 subsets of Sea-thru dataset \cite{seathur2019akkaynak}.}
	\label{tab:seathru}
	\centering
	\vspace{-2mm}
	\begin{tabular}{c||l|ccccccccc}
		\toprule
		Models    & Training Data     & $RMSE$$\downarrow$    &  $RMSE_{log}$$\downarrow$ & $A.Rel$$\downarrow$   & $S.Rel$$\downarrow$    & $log_{10}$$\downarrow$& $SI_{log}$$\downarrow$ & $\delta_1$$\uparrow$     & $\delta_2$$\uparrow$     & $\delta_3$$\uparrow$     \\ \midrule
		\multirow{3}{*}{IEBins \cite{iebins}}      & KITTI       & 4.217          & 1.072          & 3.648          & 25.007         & 0.427          & 44.031          & 0.159          & 0.311          & 0.417          \\
		& NYU Depthv2 & 3.287          & 0.901          & \textbf{0.814} & \textbf{2.373} & 0.357          & 44.753          & 0.151          & 0.350          & 0.489          \\
		& Atlantis    & \textbf{1.597} & \textbf{0.425} & 1.687          & 13.766         & \textbf{0.139} & \textbf{41.090} & \textbf{0.425} & \textbf{0.762} & \textbf{0.919} \\ \midrule
		
		\multirow{3}{*}{VA-DepthNet \cite{vadepthnet}} & KITTI       & 7.842          & 1.326          & 5.999          & 76.830         & 0.555          & 31.574          & 0.025          & 0.129          & 0.257          \\
		& NYU Depthv2 & 2.969          & 0.777          & \textbf{0.969} & \textbf{2.626} & 0.315          & 38.286          & 0.143          & 0.279          & 0.494          \\
		& Atlantis    & \textbf{1.204} & \textbf{0.292} & 1.781          & 19.937         & \textbf{0.086} & \textbf{28.739} & \textbf{0.648} & \textbf{0.939} & \textbf{0.985} \\\bottomrule
	\end{tabular}
	%\vspace{-3mm}
\end{table*}

\begin{table*}[!t]\footnotesize
	\caption{Quantitative comparisons on real underwater images from SQUID dataset \cite{squid2020berman}.}
	\label{tab:squid}
	\centering
	\vspace{-2mm}
	\begin{tabular}{c||l|ccccccccc}
		\toprule
		Models    & Training Data     & $RMSE$$\downarrow$    &  $RMSE_{log}$$\downarrow$ & $A.Rel$$\downarrow$   & $S.Rel$$\downarrow$    & $log_{10}$$\downarrow$& $SI_{log}$$\downarrow$ & $\delta_1$$\uparrow$     & $\delta_2$$\uparrow$     & $\delta_3$$\uparrow$     \\ \midrule
		\multirow{3}{*}{IEBins \cite{iebins}}      & KITTI       & 7.353          & 0.780          & 1.059          & 9.476          & 0.289          & 52.793          & 0.207          & 0.412          & 0.581          \\
		& NYU Depthv2 & 8.839          & 1.674          & 0.740          & 6.532          & 0.692          & 47.271          & 0.013          & 0.041          & 0.094          \\
		& Atlantis    & \textbf{2.896} & \textbf{0.296} & \textbf{0.263} & \textbf{0.992} & \textbf{0.100} & \textbf{29.209} & \textbf{0.615} & \textbf{0.870} & \textbf{0.951} \\ \midrule
		
		\multirow{3}{*}{VA-DepthNet \cite{vadepthnet}} & KITTI       & 8.753          & 0.827          & 1.299          & 12.381         & 0.328          & 38.362          & 0.148          & 0.308          & 0.461          \\
		& NYU Depthv2 & 8.274          & 1.349          & 0.657          & 5.747          & 0.558          & 35.518          & 0.042          & 0.112          & 0.205          \\
		& Atlantis    & \textbf{2.666} & \textbf{0.239} & \textbf{0.204} & \textbf{0.703} & \textbf{0.082} & \textbf{23.337} & \textbf{0.705} & \textbf{0.915} & \textbf{0.970} \\ \bottomrule
	\end{tabular}
	%\vspace{-3mm}
\end{table*}

\begin{table*}[!t]\footnotesize
	\caption{Quantitative comparisons of VA-DepthNet \cite{vadepthnet} performance on Sea-thru \cite{seathur2019akkaynak} and SQUID \cite{squid2020berman} datasets, trained on GAN-Based dataset and Atlantis.}
	\label{tab:gan}
	\centering
	\setlength{\tabcolsep}{0.2cm}
		
	\vspace{-2mm}
	\begin{tabular}{c||c|l|ccccccccc}
		\toprule
		Model   & Test Sets  & Training Data   & $RMSE$$\downarrow$    &  $RMSE_{log}$$\downarrow$ & $A.Rel$$\downarrow$   & $S.Rel$$\downarrow$    & $log_{10}$$\downarrow$& $SI_{log}$$\downarrow$ & $\delta_1$$\uparrow$     & $\delta_2$$\uparrow$     & $\delta_3$$\uparrow$     \\ \hline
		\multirow{6}{*}{VA-DepthNet \cite{vadepthnet}}    & \multirow{3}{*}{Sea-thru}  & NYU Depthv2 & 2.969          & 0.777          & \textbf{0.969} & \textbf{2.626} & 0.315          & 38.286          & 0.143          & 0.279          & 0.494          \\
		&& GAN-based  & 2.062          & 0.557          & 1.326          & 6.133          & 0.218          & \textbf{28.475}          & 0.164          & 0.436          & 0.751          \\
		&& Atlantis    & \textbf{1.204} & \textbf{0.292} & 1.781          & 19.937         & \textbf{0.086} & 28.739 & \textbf{0.648} & \textbf{0.939} & \textbf{0.985} \\ \cline{2-12}
		
		&\multirow{3}{*}{SQUID}  & NYU Depthv2 & 8.274          & 1.349          & 0.657          & 5.747          & 0.558          & 35.518          & 0.042          & 0.112          & 0.205          \\
		&& GAN-based   & 6.473          & 0.833          & 0.563          & 3.818          & 0.333          & 34.218          & 0.128          & 0.278          & 0.461          \\
		&& Atlantis    & \textbf{2.666} & \textbf{0.239} & \textbf{0.204} & \textbf{0.703} & \textbf{0.082} & \textbf{23.337} & \textbf{0.705} & \textbf{0.915} & \textbf{0.970} \\ \bottomrule
	\end{tabular}
	\vspace{-3mm}
\end{table*}

\section{More Qualitative Results}
We provide more qualitative results of UIEB \cite{uieb2019li} dataset in Figures \ref{fig:uieb1} to \ref{fig:uieb7}. The results highlight a significant domain gap in the depth estimates produced by pretrained terrestrial models across all four methods. This gap is evident in unclear scene layouts, ambiguous depth assignments, and inaccurate distance estimation for water bodies, often accompanied by severe artifacts. For clear underwater images (\eg, Seahorse images in Figure \ref{fig:uieb1} and Tank image in Figure \ref{fig:uieb2}), some pretrained models struggle to distinguish foreground objects from the background. The challenge intensifies in dimly lit scenes (\eg, the 4th image in Figure \ref{fig:uieb2}), where models frequently fail to produce plausible depths. In contrast, models trained on our Atlantis dataset show a marked improvement. They accurately estimate depths, preserve scene layouts, and create distinct edges in depth maps. Water bodies are correctly identified as distant, and foreground objects are more prominently featured, which is crucial for applications like Autonomous Underwater Vehicle (AUV) navigation.

Further, we provide more visual results from the SQUID dataset \cite{squid2020berman} in Figures \ref{fig:squid1} to \ref{fig:squid3}. This dataset poses greater challenges due to increased turbidity and color cast. Pretrained models generally fail to estimate depths accurately in many scenes (\eg, the 1st image in Figure \ref{fig:squid1}, the 2nd image in Figure \ref{fig:squid2} and most images in Figure \ref{fig:squid3}). However, models trained on Atlantis significantly outperform their pretrained versions, yielding plausible depth maps with better scene layout preservation and object discrimination. Notably, in complex cases like those in Figure \ref{fig:squid3}, depths estimated by models trained on Atlantis occasionally appear more reliable than the dataset's reference depth maps, derived from stereo pairs.

These results collectively underscore the effectiveness and generalization capability of Atlantis in enhancing the performance of terrestrial depth models for underwater depth estimation, offering a straightforward and effective solution for this challenging task.

\section{More Enhancement Results}
We provide more visual results of Sea-thru \cite{seathur2019akkaynak} enhancement utilizing the depth estimates by models trained on Atlantis in Figure \ref{fig:downstream1}. Similar to the results illustrated in the main paper, the appealing visual results of enchanced images confirms the effectiveness and the practical utility of our dataset in assisting underwater image enhancement.

\section{Limitation and Future Work}
While our Atlantis dataset has brought promising improvements in underwater depth estimation, it's important to recognize that this is just the initial version, featuring a relatively smaller sample size compared to KITTI \cite{kitti} and NYU Depthv2 \cite{nyudepthv2}. Currently, Atlantis comprises only 3,200 data pairs, generated using a limited set of 700 underwater images for the \textit{Depth2Underwater} ControlNet training and 400 outdoor depth maps for underwater image generation. Despite its efficacy, there are substantial opportunities for enhancing the dataset's quality and diversity, \eg, incorporating a broader range of underwater images for ControlNet pretraining and generating more varied data. Although we currently employ relative depth for its convenience and compatibility with state-of-the-art depth models, exploring the integration of absolute metric depth (potentially using diverse depth sources such as LiDAR point clouds) in the whole data generation pipeline is a promising avenue, which remains as our future work.

\begin{figure*}[t]\small
	\centering
	\includegraphics[width=\linewidth]{figures/supp/sample1.pdf}
	\includegraphics[width=\linewidth]{figures/supp/sample2.pdf}
	\vspace{-6mm}
	\caption{Samples from Atlantis, demonstrating diverse variations in scene content, lighting conditions, and color casts, corresponding to the same scene layout as indicated by the conditioning terrestrial depth map.}
	\label{fig:sample}
	\vspace{-5mm}
\end{figure*}

\begin{figure*}[!t]\small
	\centering
	\setlength{\tabcolsep}{1pt}
	
	% [inline block 0: 10 envs, 83152 chars -> data_tex | \begin{tabular}{ccccccc} 		\toprule...]

	\vspace{-3mm}
	\caption{Qualitative results on SQUID \cite{squid2020berman} dataset. K, N and A denote pretrained models of KITTI \cite{kitti}, NYU Depthv2 \cite{nyudepthv2} datasets and the model trained on our Atlantis dataset. Models trained on Atlantis get the best visual results. Please zoom in for details.} 
	\label{fig:squid3}
	\vspace{-5mm}
\end{figure*}

\begin{figure*}[t]\small
	\centering
	\includegraphics[width=\linewidth]{figures/supp/downstream1.pdf}
	\includegraphics[width=\linewidth]{figures/supp/downstream2.pdf}
	\vspace{-6mm}
	\caption{Qualitative results of the improved depth result applied to Sea-thru algorithm \cite{seathur2019akkaynak} on images from UIEB dataset \cite{uieb2019li}. Enhancement outputs well show the practical utility of Atlantis on training depth models for reliable underwater depth estimation.}
	\label{fig:downstream1}
	\vspace{-5mm}
\end{figure*}
